# Supplementary material for: First order corrections to black hole thermodynamics: a simple approach enhanced
Source: arXiv:2312.07127 ancillary file (2024-11-18)
Supplement: Supplementary file 1 [file attached_notebook_v1.pdf]

Note : The file uses the package "diffgeoM.m", which can be downloaded from : "<https://github.com/bryango/diffgeoM>".

## \* Example I: The (enhanced) simple approach to the BH thermodynamics with $R^2$ corrections.

```
Quit[];
```

### 0. The unperturbed BH solution:

```
In[1]:= coord = {t, r, ψ, θ, ϕ};
$Assumptions = And[t ∈ Reals, M ∈ Reals, r ∈ Reals, r > 0,
    θ < ϕ < 2 π, 0 < ψ < π, 0 < θ < π, M > 0, Λ < 0, Λe < 0, l > 0, le > 0];
metricsign = -1;
metric = DiagonalMatrix[
    {- (f[r]), 1 / (f[r]), r^2, r^2 * (Sin[ψ])^2, r^2 * (Sin[ψ] * Sin[θ])^2}];
<< "D:\\diffgeoM.wl"
rieθ = lower[Riemann, {4}];
```

```
In[7]:= ff[r_] = 1 - mu / r^2 - r^2 Λe / 6;
sr[var_] := Normal[Series[var, {α, 0, 1}]];
srθ[var_] := Normal[Series[var, {α, 0, 0}]];
```

( ff[r] is the concrete expression of f[r]. We make the substitution f->ff when it is needed. )

```
In[10]:= mu0 = rh0^2 - (rh0^4 Λe) / 6;
tem = 1 / (2 π rh0) - (rh0 Λe) / (6 π);
```

We use `rh0` to represent the barred quantity  $\bar{\text{rh}}$  in our paper.

### 1. The effective cosmological constant:

The formula is  $\Lambda_e - \Lambda = \frac{k-D1}{2 D1} \propto L_k$ .

```
In[12]:= rHcR2 =
  α * contract[contract[rie0**rie0, {3, 5}, {4, 6}], {1, 3}, {2, 4}] /. f → ff /.
  {mu → 0, q → 0};
Λe - Λ - (k - d1) / (2 d1) * % /. {k → 4, d1 → 5, Λ → Λe (1 + α * b1 Λe)} // sr;
Solve[% == 0, b1];
Λf = Λe (1 + α b1 Λe) /. %[[1]]
Λef = Λ (1 - α b1 Λ) /. %[[1]]
```

Out[15]=

$$\Lambda e \left( 1 + \frac{\alpha \Lambda e}{9} \right)$$

Out[16]=

$$\Lambda \left( 1 - \frac{\alpha \Lambda}{9} \right)$$

Above,  $\Lambda ef$  is the expression of  $\Lambda e$  as a function of  $\Lambda$ , while  $\Lambda f$  is the expression of  $\Lambda$  as a function of  $\Lambda e$ .

## 2. The free energy at first order in $\alpha$ :

According to the simple approach, at first order in  $\alpha$ , the part  $\int R-2 \Lambda e$  of the Euclidean integral can be approximately by

In[17]=

$$\ln z_{EH} = \beta \left( -2 \pi^2 r h \theta^2 - \frac{1}{3} \pi^2 r h \theta^4 \Lambda e \right);$$

The higher curvature part  $\alpha \int L_{hd}$  and the part  $\int 2(\Lambda e - \Lambda)$  can be calculated by inserting the unperturbed metric into them. Before doing this, we should compute the factor  $\sqrt{g_{tt}(BH)/g_{tt}(AdS)}$  (denoted as m12b below) needed to regularize the action:

In[18]=

```
ff[r] / (ff[r] /. {mu → 0});
Series[(Sqrt[%] /. r → 1/ep), {ep, 0, 4}] // Normal;
m12b = % /. ep → 1/rc // sr
```

Out[20]=

$$1 + \frac{3 \mu}{rc^4 \Lambda e}$$

Then, we can evaluate  $\alpha \int L_{hd} + k1 \int 2(\Lambda e - \Lambda)$  together. Here we use the symbol k1 to trace the contribution of  $\int 2(\Lambda e - \Lambda)$ . When k1=1, we get the needed results in the paper.

```

In[21]:= rHd1 =
  α * contract[contract[rie0**rie0, {3, 5}, {4, 6}], {1, 3}, {2, 4}] /. f → ff;
rHd0 = 2 ((Λe) - (Λ)) /. Λ → Λf // sr;
rHd1 + k1 rHd0 // Simplify;
ind = (%) * 2 Pi^2 r^3 /. {Λ → Λf, f → ff} // Simplify // sr;
int[r_] = Integrate[%, r];
int[rc] - int[rh] // Simplify;
rInt = % // Simplify // sr;
rInt - m12b * (int[rc] /. {mu → 0, q → 0}) // Simplify // sr;
Limit[%, rc → Infinity] // Expand // sr;
lnzL4 = β % /. {rh → rh0, mu → mu0} // sr

```

$$\text{Out[30]} = \frac{1}{18} \alpha \beta \left( 648 \pi^2 - 246 \pi^2 \text{rh0}^2 \Lambda e + 6 k1 \pi^2 \text{rh0}^2 \Lambda e + 13 \pi^2 \text{rh0}^4 \Lambda e^2 + k1 \pi^2 \text{rh0}^4 \Lambda e^2 \right)$$

The total partition function and the free energy for the perturbed BH:

```

In[31]:= lnzPd = \frac{1}{16 \text{Pi}} (\lnzEH + \lnzL4);
freePd = -1 / \beta * lnzPd /. k1 → 1 // Simplify // sr

```

$$\text{Out[32]} = \frac{1}{48} \pi \left( 6 \text{rh0}^2 + \text{rh0}^4 \Lambda e \right) + \frac{1}{144} \pi \alpha \left( -324 + 120 \text{rh0}^2 \Lambda e - 7 \text{rh0}^4 \Lambda e^2 \right)$$

### 3. The thermodynamic quantities followed from the free energy.

The expressions for  $\text{rh0}^{(1,0)} [T, \Lambda e]$ ,  $\text{rh0}^{(0,1)} [T, \Lambda e]$  is given below. They are useful when taking the derivative of the free energy with respect to  $T$  and  $\Lambda e$ , according to the chain rule of calculus.

```

In[36]:= Outer[D, {T - (tem /. rh0 → rh0[T, Λe]) == 0}, {T, Λe}];
Solve[%%[[1]], {rh0^{(1,0)} [T, Λe], rh0^{(0,1)} [T, Λe]}];
sub = %[[1]] /. {rh0[T, Λe] → rh0}

```

$$\text{Out[38]} = \left\{ \text{rh0}^{(1,0)} [T, \Lambda e] \rightarrow -\frac{6 \pi \text{rh0}^2}{3 + \text{rh0}^2 \Lambda e}, \text{rh0}^{(0,1)} [T, \Lambda e] \rightarrow -\frac{\text{rh0}^3}{3 + \text{rh0}^2 \Lambda e} \right\}$$

The entropy for the perturbed BH is computed by the formula  $S = d F / d T$ :

In[39]:=

```
entrPd =
  -D[(freePd /. rh0 -> rh0[T, Δe]), T] /. sub /. {rh0[T, Δe] -> rh0} // Simplify // sr
```

Out[39]:=

$$\frac{\pi^2 \text{rh0}^3}{2} + \frac{\pi^2 \text{rh0}^3 \alpha (60 \Delta e - 7 \text{rh0}^2 \Delta e^2)}{6 (3 + \text{rh0}^2 \Delta e)}$$

The energy of the BH is calculated from the formula  $M=F+TS$ .

In[41]:=

```
massPd = freePd + tem * entrPd // sr
```

Out[41]:=

$$\frac{1}{16} (6 \pi \text{rh0}^2 - \pi \text{rh0}^4 \Delta e) + \frac{\alpha (-324 \pi + 252 \pi \text{rh0}^2 \Delta e - 75 \pi \text{rh0}^4 \Delta e^2 + 7 \pi \text{rh0}^6 \Delta e^3)}{48 (3 + \text{rh0}^2 \Delta e)}$$

Note that we can also get the Wald entropy for the perturbed BH at first order in  $\alpha$ , from the unperturbed solution. It is given by a function of  $r_h$ .

In[42]:=

```
entrWd = 2 Pi^2 rh^3 / 4 ( 1 - 4 α * rie0[[1, 2, 1, 2]] ) /. {f -> ff} /. r -> rh // sr;
% /. mu -> mu0 /. rh0 -> rh // sr
```

Out[43]:=

$$\frac{\pi^2 \text{rh}^3}{2} - \frac{2}{3} \pi^2 \text{rh} \alpha (-9 + \text{rh}^2 \Delta e)$$

Requiring  $\text{entr} == \text{entrWd}$ , we can derive a relation between  $\text{rh0}$  and  $\text{rh}$ . This relation is useful, if one intends to use the horizon radius  $\text{rh}$  of the perturbed metric as a variable, instead of  $\text{rh0}$ .

In[44]:=

```
entrWd - entrPd /. mu -> mu0 /. rh0 -> rh (1 + α b1) /. Δ -> Δf // sr;
Solve[% == 0, b1] // Simplify;
rh0f = rh (1 + α b1) /. %[[1]]
```

Out[46]:=

$$\text{rh} \left( 1 + \frac{\alpha (-6 + \text{rh}^2 \Delta e)^2}{3 \text{rh}^2 (3 + \text{rh}^2 \Delta e)} \right)$$

#### 4. The conventional and extended first law of BH thermodynamics.

Now we verify the conventional first law of BH thermodynamics:  $dM - TdS=0$ , using  $\text{rh0}$  as the variable.

```
In[47]:= diff[va_] := Outer[D, {va}, {rh0}][[1]];
diff[massPd] - tem * diff[entrPd] // sr
```

```
Out[48]= {0}
```

Next, we construct the **extended first law** of BH thermodynamics:  $dM = TdS + \Theta d(\Lambda e) + U_\alpha d\alpha$ .

First, we calculate the conjugate quantities associated with  $\Lambda e$  and  $\alpha$ . The conjugate quantity  $\Theta_e$  associated to  $\Lambda e$  is calculated below.

```
In[49]:= freeqtF = freePd /. rh0 -> rh0[T, \Lambda e];
D[%, \Lambda e] /. sub /. rh0[T, \Lambda e] -> rh0 // Simplify;
vth\Lambda e = % // Simplify // sr
```

```
Out[51]= - \frac{\pi rh0^4}{16} + \frac{\pi \alpha (360 rh0^2 - 162 rh0^4 \Lambda e + 14 rh0^6 \Lambda e^2)}{144 (3 + rh0^2 \Lambda e)}
```

The conjugate quantity  $U_\alpha$  associated to  $\alpha$  is calculated below:

```
In[52]:= vthAlpha = D[freePd, \alpha] // Simplify // sr
```

```
Out[52]= - \frac{1}{144} \pi (324 - 120 rh0^2 \Lambda e + 7 rh0^4 \Lambda e^2)
```

Now verify the extended first law:  $dM = TdS + \Theta d(\Lambda e) - U_\alpha d\alpha$ . We use the parameters  $rh0$ ,  $\Lambda e$  and  $\alpha$  as the independent variables.

```
In[53]:= diff[tquant_] := Outer[D, {tquant}, {rh0, \Lambda e, \alpha}];
```

```
In[54]:= diff[massPd] - tem * diff[entrPd] - vth\Lambda e * diff[\Lambda e] - vthAlpha * diff[\alpha] // sr;
Table[%[[1]][[i]] == 0, {i, 1, 2}]
Series[%[[1]][[3]], {\alpha, 0, 0}] == 0 // Simplify
```

```
Out[55]= {True, True}
```

```
Out[56]= True
```

(  $U_\alpha d\alpha$  is at first order in  $\alpha$ , so  $U_\alpha$  should be understood as an expression at zero order in  $\alpha$ .)

## 5.The summary of the derived expressions:

The thermodynamic quantities are expressed using the following variables:

the horizon radius  $rh$  of the perturbed BH, the AdS radius  $l$  and the coupling  $\alpha$ , for a better comparison with those results in Sec.4 of arXiv:2205.15593.

In[57]:= `massPd /. rh0 -> rhOf /. Δe -> Δef /. Δ -> -6 / l^2 // sr`

$$\text{Out[57]} = \frac{1}{16} \left( 6 \pi rh^2 + \frac{6 \pi rh^4}{l^2} \right) + \frac{(3 l^4 \pi + 12 l^2 \pi rh^2 + 10 \pi rh^4) \alpha}{4 l^4}$$

In[58]:= `tem /. rh0 -> rhOf /. Δe -> Δef /. Δ -> -6 / l^2 // sr`

$$\text{Out[58]} = \frac{1}{2 \pi rh} + \frac{rh}{l^2 \pi} - \frac{2 (3 l^4 + 6 l^2 rh^2 + 2 rh^4) \alpha}{3 l^4 \pi rh^3}$$

In[59]:= `entrPd /. rh0 -> rhOf /. Δe -> Δef /. Δ -> -6 / l^2 // sr`

$$\text{Out[59]} = \frac{\pi^2 rh^3}{2} + \frac{2 \pi^2 (3 l^2 rh + 2 rh^3) \alpha}{l^2}$$

In[60]:= `vthΔe /. rh0 -> rhOf /. Δe -> Δef /. Δ -> -6 / l^2 // sr`

$$\text{Out[60]} = -\frac{\pi rh^4}{16} - \frac{\pi (2 l^2 rh^2 + rh^4) \alpha}{12 l^2}$$

In[61]:= `vthAlpha /. rh0 -> rhOf /. Δe -> Δef /. Δ -> -6 / l^2 // sr0 // Simplify`

$$\text{Out[61]} = -\frac{\pi (9 l^4 + 20 l^2 rh^2 + 7 rh^4)}{4 l^4}$$

Note that the thermodynamic quantities can be re-expressed using any of these sets of variables :  $\{rh, \Delta e, \alpha\}$ ,  $\{rh0, \Delta e, \alpha\}$ , or  $\{rh0, \Delta, \alpha\}$ , by simply using the following substitutions:  $rh0 \rightarrow rhOf$ ,  $\Delta e \rightarrow \Delta ef$ , and  $\Delta \rightarrow \Delta f$ .

## \* Example II: The (enhanced) simple approach to the charged BH thermodynamics with four-derivative corrections.

In[23]:= `Quit[];`

0. The unperturbed BH solution: (which includes the gravitational and the

## electromagnetic sectors)

```

In[1]:= coord = {t, r, ψ, θ, ϕ};
$Assumptions = And[t ∈ Reals, M ∈ Reals, r ∈ Reals, r > 0,
  0 < ϕ < 2 π, 0 < ψ < π, 0 < θ < π, M > 0, Δ < 0, Δe < 0, l > 0, le > 0];
metricsign = -1;
metric = DiagonalMatrix[
  {- (f[r]), 1 / (f[r]), r^2, r^2 * (Sin[ψ])^2, r^2 * (Sin[ψ] * Sin[θ])^2}];
<< "D:\\diffgeoM.wl"
rieθ = lower[Riemann, {4}];

```

```

In[7]:= ff[r_] = 1 +  $\frac{q^2}{4 r^4} - \frac{\mu}{r^2} - \frac{r^2 \Delta e}{6}$ ;

au = {-  $\frac{\sqrt{3}}{2} (q / r^2)$ , 0, 0, 0, 0};

fuv = covariant[au] - Transpose[covariant[au], {2, 1}] // Simplify;
fuvup = raise[%, {1, 2}] // Simplify;
sr[var_] := Normal[Series[var, {ε, 0, 1}]];
srθ[var_] := Normal[Series[var, {ε, 0, 0}]];

```

( ff[r] is the concrete expression of f[r]. We make the substitution f->ff when it is needed. )

To use the simple approach, one should be familiar with the thermodynamics of the original BH:

```

In[13]:= muθ =  $\frac{q^2}{4 r h \theta^2} + r h \theta^2 - \frac{r h \theta^4 \Delta e}{6}$ ;

tem = -  $\frac{q^2}{8 \pi r h \theta^5} + \frac{1}{2 \pi r h \theta} - \frac{r h \theta \Delta e}{6 \pi}$ ;

phiθ =  $\frac{\sqrt{3}}{2} \left( \frac{q}{r h \theta^2} \right)$ ;

Qθ =  $\frac{1}{8} \sqrt{3} \pi q$ ;

freeθ =  $\frac{\pi r h \theta^2}{8} + \frac{\pi r h \theta^4 \Delta e}{48} - \frac{\pi q^2}{32 r h \theta^2}$ ;

freeqtθ =  $\frac{1}{8} \pi r h \theta^2 + \frac{1}{48} \pi r h \theta^4 \Delta e + \frac{5 \pi q^2}{32 r h \theta^2}$ ;

```

Above, we use the symbol  $\text{rh}\theta$  to represent the barred quantity  $\bar{r}_h$  in our paper.

## 1. The effective cosmological constant:

The formula is  $\Lambda_e - \Lambda = \frac{2m-D1}{D1} \alpha F$ .

```
In[19]:= rHcR2 =  $\epsilon$  * c1 contract[contract[rie0**rie0, {3, 5}, {4, 6}], {1, 3}, {2, 4}] /.
      f -> ff /. {mu -> 0, q -> 0};
      (2 m - d1) / (2 d1) * % /. {m -> 2, d1 -> 5} // sr;
       $\Delta$ ef =  $\Delta$  + (% /.  $\Delta$ e ->  $\Delta$ ) // sr
       $\Delta$ f =  $\Delta$ e - %% // sr
```

```
Out[21]= 
$$\Lambda - \frac{1}{9} c1 \in \Lambda^2$$

```

```
Out[22]= 
$$\Delta e + \frac{1}{9} c1 \in \Delta e^2$$

```

Above,  $\Delta$ ef is the expression of  $\Delta$ e as a function of  $\Delta$ , while  $\Delta$ f is the expression of  $\Delta$  as a function of  $\Delta$ e.

## 2. The free energy at first order in $\epsilon$ :

According to the simple approach, at first order in  $\epsilon$ , the part  $\int R - 2 \Lambda e - \frac{1}{4} F^2$  of the Euclidean integral can be approximately by the known form:

```
In[23]:= lnzEH =  $\beta$   $\left( -\frac{5 \pi^2 q^2}{2 rh\theta^2} - 2 \pi^2 rh\theta^2 - \frac{1}{3} \pi^2 rh\theta^4 \Delta e \right);$ 
```

The above formula is that of the ensemble depending on T and q. The higher derivative part  $\epsilon \int L_{hd}$  and the part  $\int 2(\Lambda_e - \Lambda)$  can be calculated by inserting the unperturbed BH solution into them. Below we use the symbol k1 to trace the contribution of  $\int 2(\Lambda_e - \Lambda)$ . When k1=1, we get the needed results in the paper.



```

In[24]:= rHd0 = 2 k1 (Λe - Λ) /. Λ → Δf // sr;
rHd1 =
  contract[contract[rie0**rie0, {3, 5}, {4, 6}], {1, 3}, {2, 4}] /. f → ff;
rHd2 = contract[rie0**fuv**fuv, {1, 5}, {2, 6}, {3, 7}, {4, 8}] /. f → ff;
contract[fuv**fuv, {1, 3}, {2, 4}] /. f → ff;
rHd3 = %^2;
rHd4 = tr[(fuv.fuvup).fuv.fuvup, {1, 2}] /. f → ff;
e = (c1 rHd1 + c2 rHd2 + c3 rHd3 + c4 rHd4) + rHd0 // Simplify;
ind = (%) * 2 Pi^2 r^3 /. {Λ → Δf, f → ff} // Simplify // sr;
int[r_] = Integrate[%, r];
int[rt] - int[rh] // Simplify;
rInt = % // Simplify // sr

```

$$\frac{1}{144 r h^8 r t^8} \pi^2 \in \left( 72 \left( -15 c_2 q^4 (r h^8 - r t^8) - 9 (2 c_3 + c_4) q^4 (r h^8 - r t^8) + \right. \right. \\ \left. \left. 4 c_2 q^2 (6 \mu r h^2 r t^2 (r h^6 - r t^6) + r h^6 r t^6 (r h^2 - r t^2) \Delta e) \right) + \right. \\ \left. c_1 \left( -1143 q^4 (r h^8 - r t^8) + 48 q^2 (90 \mu r h^2 r t^2 (r h^6 - r t^6) + r h^6 r t^6 (r h^2 - r t^2) \Delta e) + \right. \right. \\ \left. \left. 16 r h^4 r t^4 (r h^4 - r t^4) (-324 \mu^2 + (-5 + k_1) r h^4 r t^4 \Delta e^2) \right) \right)$$

```

In[35]:= ff[r] / (ff[r] /. {mu → 0, q → 0});
Series[Sqrt[%] /. r → 1/ep), {ep, 0, 4}] // Normal;
m12b = % /. ep → 1/rt // sr

```

$$\text{Out[37]= } 1 + \frac{3 \mu}{r t^4 \Delta e}$$

```

In[38]:= rInt - m12b * (int[rt] /. {mu → 0, q → 0}) // Simplify // sr;
Limit[%, rt → Infinity] // Expand // sr;
lnzL4 = β % /. {rh → rh0, mu → mu0} // sr;

```

```

In[41]:= lnzPd = \frac{1}{16 \pi} (\lnzEH + \lnzL4);
freeqtPd = -1/β * lnzPd /. k1 → 1 // Simplify // sr

```

$$\text{Out[42]= } \frac{15 \pi q^2 + 12 \pi r h^4 + 2 \pi r h^6 \Delta e}{96 r h^2} + \frac{1}{2304 r h^8} \\ \in \left( -387 c_1 \pi q^4 - 648 c_2 \pi q^4 - 1296 c_3 \pi q^4 - 648 c_4 \pi q^4 + 1728 c_1 \pi q^2 r h^4 + 1728 c_2 \pi q^2 r h^4 - \right. \\ \left. 5184 c_1 \pi r h^8 - 192 c_1 \pi q^2 r h^6 \Delta e + 1920 c_1 \pi r h^{10} \Delta e - 112 c_1 \pi r h^{12} \Delta e^2 \right)$$

Notice the free energy is that of the ensemble depending on T and q.

### 3. The thermodynamic quantities followed from the free energy.

The expressions for  $\text{rh}\theta^{(1,0)}[T, q]$ ,  $\text{rh}\theta^{(0,1)}[T, q]$  is given below. They are useful when taking the derivatives of the free energy with respect to  $T$  and  $q$  by the chain rule of calculus.

```
In[43]:= Outer[D, {T - (tem /. rh0 -> rh0[T, q]) == 0}, {T, q}];
Solve[%[[1]], {rh0^(1,0)[T, q], rh0^(0,1)[T, q]}];
sub = %[[1]] /. {rh0[q, T] -> rh0};
```

Calculate the electrostatic potential:

```
In[46]:= phiPd = D[(freeqtPd /. rh0 -> rh0[T, q]), q] / (1/8 sqrt[3] pi) /. sub /.
rh0[T, q] -> rh0 // Simplify // sr
```

```
Out[46]= 
$$\frac{\sqrt{3} q}{2 \text{rh}\theta^2} + \frac{1}{8 \sqrt{3} \text{rh}\theta^8 (-15 q^2 + 12 \text{rh}\theta^4 + 4 \text{rh}\theta^6 \Delta e)}$$


$$\in (129 c_1 q^5 + 216 c_2 q^5 + 432 c_3 q^5 + 216 c_4 q^5 - 804 c_1 q^3 \text{rh}\theta^4 -$$


$$1152 c_2 q^3 \text{rh}\theta^4 - 1728 c_3 q^3 \text{rh}\theta^4 - 864 c_4 q^3 \text{rh}\theta^4 + 1152 c_1 q \text{rh}\theta^8 +$$


$$1152 c_2 q \text{rh}\theta^8 - 76 c_1 q^3 \text{rh}\theta^6 \Delta e - 288 c_2 q^3 \text{rh}\theta^6 \Delta e - 576 c_3 q^3 \text{rh}\theta^6 \Delta e -$$


$$288 c_4 q^3 \text{rh}\theta^6 \Delta e - 384 c_1 q \text{rh}\theta^{10} \Delta e + 384 c_2 q \text{rh}\theta^{10} \Delta e + 32 c_1 q \text{rh}\theta^{12} \Delta e^2)$$

```

Calculate the entropy from the formula  $S = dF/dT$ :

```
In[47]:= entrPd =
-D[(freeqtPd /. rh0 -> rh0[T, q]), T] /. sub /. {rh0[T, q] -> rh0} // Simplify // sr
```

```
Out[47]= 
$$\frac{\pi^2 \text{rh}\theta^3}{2} +$$


$$\left( \pi^2 \in (387 c_1 q^4 + 648 c_2 q^4 + 1296 c_3 q^4 + 648 c_4 q^4 - 864 c_1 q^2 \text{rh}\theta^4 - 864 c_2 q^2 \text{rh}\theta^4 + 48 c_1 q^2 \text{rh}\theta^6 \Delta e + 480 c_1 \text{rh}\theta^{10} \Delta e - 56 c_1 \text{rh}\theta^{12} \Delta e^2) \right) / (-180 q^2 \text{rh}\theta^3 + 48 \text{rh}\theta^7 (3 + \text{rh}\theta^2 \Delta e))$$

```

The energy of the BH is calculated from the formula  $M = F + TS$ .

In[48]:= **massPd = freeqPd + tem \* entrPd // sr**

Out[48]=

$$\frac{3 \pi q^2 + 12 \pi rh\theta^4 - 2 \pi rh\theta^6 \Delta e}{32 rh\theta^2} + \epsilon \left( - \left( \pi \left( 3 q^2 - 12 rh\theta^4 + 4 rh\theta^6 \Delta e \right) \left( 387 c_1 q^4 + 648 c_2 q^4 + 1296 c_3 q^4 + 648 c_4 q^4 - 864 c_1 q^2 rh\theta^4 - 864 c_2 q^2 rh\theta^4 + 48 c_1 q^2 rh\theta^6 \Delta e + 480 c_1 rh\theta^{10} \Delta e - 56 c_1 rh\theta^{12} \Delta e^2 \right) \right) / \left( 288 rh\theta^8 \left( -15 q^2 + 12 rh\theta^4 + 4 rh\theta^6 \Delta e \right) \right) + \frac{1}{2304 rh\theta^8} \left( -387 c_1 \pi q^4 - 648 c_2 \pi q^4 - 1296 c_3 \pi q^4 - 648 c_4 \pi q^4 + 1728 c_1 \pi q^2 rh\theta^4 + 1728 c_2 \pi q^2 rh\theta^4 - 5184 c_1 \pi rh\theta^8 - 192 c_1 \pi q^2 rh\theta^6 \Delta e + 1920 c_1 \pi rh\theta^{10} \Delta e - 112 c_1 \pi rh\theta^{12} \Delta e^2 \right) \right)$$

Note that we can also get the Wald entropy for the perturbed BH at first order in  $\epsilon$ , from the unperturbed solution. It is given by a function of  $r_h$ .

In[49]:=

**entrWd =**  
**2 Pi^2 rh^3 / 4 ( 1 - \epsilon \* ( 4 c1 rie0[[1, 2, 1, 2]] + 2 c2 fuv[[1, 2]] fuv[[1, 2]] ) ) /. {f -> ff} /. r -> rh // sr**

Out[49]=

$$\frac{\pi^2 rh^3}{2} + \frac{\epsilon \left( -15 c_1 \pi^2 q^2 - 9 c_2 \pi^2 q^2 + 18 c_1 \mu \pi^2 rh^2 + c_1 \pi^2 rh^6 \Delta e \right)}{3 rh^3}$$

Requiring  $\text{entr} == \text{entrWd}$ , we can derive a relation between  $rh0$  and  $rh$ . This relation is useful, if one intends to use the horizon radius  $rh$  of the perturbed metric as a variable, instead of  $rh0$ .

In[50]:=

**(entrWd - entrPd) /. mu -> mu0 /. rh0 -> rh \* (1 + \epsilon b1) // sr;**  
**Solve[% == 0, b1];**  
**rh0f = rh (1 + \epsilon b1) /. %[[1]] // sr**

Out[52]=

$$rh + \left( \epsilon \left( 81 c_1 q^4 - 36 c_2 q^4 - 432 c_3 q^4 - 216 c_4 q^4 - 240 c_1 q^2 rh^4 + 144 c_2 q^2 rh^4 + 288 c_1 rh^8 - 32 c_1 q^2 rh^6 \Delta e - 48 c_2 q^2 rh^6 \Delta e - 96 c_1 rh^{10} \Delta e + 8 c_1 rh^{12} \Delta e^2 \right) \right) / \left( 6 rh^5 \left( -15 q^2 + 12 rh^4 + 4 rh^6 \Delta e \right) \right)$$

#### 4. The conventional and extended first law of BH thermodynamics.

Now we verify the **conventional first law** of BH thermodynamics:  $dM = TdS + \phi dQ$ , using  $rh0$  and  $q$  as the variables.

```
In[53]:= diff[va_] := Outer[D, {va}, {rh0, q}][[1]];
diff[massPd] - tem * diff[entrPd] - phiPd diff[Q0] // sr
```

```
Out[54]= {0, 0}
```

Next, we construct the **extended first law** of BH thermodynamics:  $dM = TdS + \phi dq + \Theta d(\Lambda e) + U_\epsilon d\epsilon$ , using  $rh0$ ,  $q$ ,  $\Lambda e$  and  $\epsilon$  as the independent variables. First, we calculate the conjugate quantities associated with  $\Lambda e$  and  $\epsilon$ . The expression for  $rh0'[\Lambda e]$  is calculated below, which is useful when taking the derivative of the free energy with respect to  $\Lambda e$ . Then the conjugate quantity  $\Theta_e$  associated to  $\Lambda e$  is given by:

```
In[55]:= D[T - (tem /. rh0 -> rh0[Λe]), Λe] == 0;
Solve[%, rh0'[Λe]] /. rh0[Λe] -> rh0;
jac = rh0'[Λe] /. %[[1]];
D[freeqtPd, Λe] + D[freeqtPd, rh0] * jac // Simplify;
vthΛe = % // Simplify // sr
```

```
Out[59]= -\frac{\pi rh0^4}{16} +
```

$$\left( \pi \in \left( -297 c_1 q^4 - 648 c_2 q^4 - 1296 c_3 q^4 - 648 c_4 q^4 - 108 c_1 q^2 rh0^4 + 864 c_2 q^2 rh0^4 + 720 c_1 rh0^8 + 33 c_1 q^2 rh0^6 \Lambda e - 324 c_1 rh0^{10} \Lambda e + 28 c_1 rh0^{12} \Lambda e^2 \right) \right) /$$

$$\left( 72 rh0^2 \left( -15 q^2 + 12 rh0^4 + 4 rh0^6 \Lambda e \right) \right)$$

The conjugate quantity  $U_\epsilon$  associated to  $\epsilon$  is calculated by:

```
In[60]:= vthEp = D[freeqtPd, ε] // Simplify // sr
```

```
Out[60]= -\frac{1}{2304 rh0^8} \pi \left( 216 \left( 3 \left( 2 c_3 + c_4 \right) q^4 + c_2 \left( 3 q^4 - 8 q^2 rh0^4 \right) \right) + \right.

$$\left. c_1 \left( 387 q^4 + 192 q^2 rh0^4 \left( -9 + rh0^2 \Lambda e \right) + 16 rh0^8 \left( 324 - 120 rh0^2 \Lambda e + 7 rh0^4 \Lambda e^2 \right) \right) \right)$$


```

Now we verify the extended first law  $dM = TdS + \phi dq + \Theta d\Lambda e + U_\epsilon d\epsilon$ :

```
In[61]:= diff[tquant_] := Outer[D, {tquant}, {rh0, q, Λe, ε}];
diff[massPd] - tem * diff[entrPd] -
  phiPd diff[Q0] - vthΛe * diff[Λe] - vthEp * diff[ε] // sr;
Table[%[[1]][[i]] == 0, {i, 1, 3}]
Series[%[[1]][[4]], {ε, 0, 0}] == 0 // Simplify
```

```
Out[63]= {True, True, True}
```

```
Out[64]= True
```

(  $U_\epsilon d\epsilon$  is at first order in  $\epsilon$  , so  $U_\epsilon$  should be understood at zero order in  $\epsilon$  . )

## 5.The summary of the derived expressions:

In[65]:=

**freeqtPd**

Out[65]=

$$\frac{15 \pi q^2 + 12 \pi \text{rh}\theta^4 + 2 \pi \text{rh}\theta^6 \Delta e}{96 \text{rh}\theta^2} + \frac{1}{2304 \text{rh}\theta^8} \\ \in \left( -387 c_1 \pi q^4 - 648 c_2 \pi q^4 - 1296 c_3 \pi q^4 - 648 c_4 \pi q^4 + 1728 c_1 \pi q^2 \text{rh}\theta^4 + 1728 c_2 \pi q^2 \text{rh}\theta^4 - \right. \\ \left. 5184 c_1 \pi \text{rh}\theta^8 - 192 c_1 \pi q^2 \text{rh}\theta^6 \Delta e + 1920 c_1 \pi \text{rh}\theta^{10} \Delta e - 112 c_1 \pi \text{rh}\theta^{12} \Delta e^2 \right)$$

In[66]:=

**massPd**  
**entrPd**  
**tem**  
**phiPd**  
**Q0**  
**vthΔe**  
**vthEp**

Out[66]=

$$\frac{3 \pi q^2 + 12 \pi \text{rh}\theta^4 - 2 \pi \text{rh}\theta^6 \Delta e}{32 \text{rh}\theta^2} + \\ \in \left( - \left( \pi \left( 3 q^2 - 12 \text{rh}\theta^4 + 4 \text{rh}\theta^6 \Delta e \right) \left( 387 c_1 q^4 + 648 c_2 q^4 + 1296 c_3 q^4 + 648 c_4 q^4 - 864 c_1 q^2 \text{rh}\theta^4 - \right. \right. \right. \\ \left. \left. \left. \text{rh}\theta^4 - 864 c_2 q^2 \text{rh}\theta^4 + 48 c_1 q^2 \text{rh}\theta^6 \Delta e + 480 c_1 \text{rh}\theta^{10} \Delta e - 56 c_1 \text{rh}\theta^{12} \Delta e^2 \right) \right) / \right. \\ \left. \left( 288 \text{rh}\theta^8 \left( -15 q^2 + 12 \text{rh}\theta^4 + 4 \text{rh}\theta^6 \Delta e \right) \right) + \frac{1}{2304 \text{rh}\theta^8} \left( -387 c_1 \pi q^4 - \right. \right. \\ \left. \left. 648 c_2 \pi q^4 - 1296 c_3 \pi q^4 - 648 c_4 \pi q^4 + 1728 c_1 \pi q^2 \text{rh}\theta^4 + 1728 c_2 \pi q^2 \text{rh}\theta^4 - \right. \right. \\ \left. \left. 5184 c_1 \pi \text{rh}\theta^8 - 192 c_1 \pi q^2 \text{rh}\theta^6 \Delta e + 1920 c_1 \pi \text{rh}\theta^{10} \Delta e - 112 c_1 \pi \text{rh}\theta^{12} \Delta e^2 \right) \right)$$

Out[67]=

$$\frac{\pi^2 \text{rh}\theta^3}{2} + \\ \left( \pi^2 \in \left( 387 c_1 q^4 + 648 c_2 q^4 + 1296 c_3 q^4 + 648 c_4 q^4 - 864 c_1 q^2 \text{rh}\theta^4 - 864 c_2 q^2 \text{rh}\theta^4 + 48 c_1 q^2 \text{rh}\theta^6 \Delta e + 480 c_1 \text{rh}\theta^{10} \Delta e - 56 c_1 \text{rh}\theta^{12} \Delta e^2 \right) \right) / \left( -180 q^2 \text{rh}\theta^3 + 48 \text{rh}\theta^7 \left( 3 + \text{rh}\theta^2 \Delta e \right) \right)$$

Out[68]=

$$-\frac{q^2}{8 \pi \text{rh}\theta^5} + \frac{1}{2 \pi \text{rh}\theta} - \frac{\text{rh}\theta \Delta e}{6 \pi}$$

Out[69]=

$$\frac{\sqrt{3} q}{2 \text{rh}\theta^2} + \frac{1}{8 \sqrt{3} \text{rh}\theta^8 (-15 q^2 + 12 \text{rh}\theta^4 + 4 \text{rh}\theta^6 \Lambda e)}$$

$$\in (129 c_1 q^5 + 216 c_2 q^5 + 432 c_3 q^5 + 216 c_4 q^5 - 804 c_1 q^3 \text{rh}\theta^4 - 1152 c_2 q^3 \text{rh}\theta^4 - 1728 c_3 q^3 \text{rh}\theta^4 - 864 c_4 q^3 \text{rh}\theta^4 + 1152 c_1 q \text{rh}\theta^8 + 1152 c_2 q \text{rh}\theta^8 - 76 c_1 q^3 \text{rh}\theta^6 \Lambda e - 288 c_2 q^3 \text{rh}\theta^6 \Lambda e - 576 c_3 q^3 \text{rh}\theta^6 \Lambda e - 288 c_4 q^3 \text{rh}\theta^6 \Lambda e - 384 c_1 q \text{rh}\theta^{10} \Lambda e + 384 c_2 q \text{rh}\theta^{10} \Lambda e + 32 c_1 q \text{rh}\theta^{12} \Lambda e^2)$$

Out[70]=

$$\frac{1}{8} \sqrt{3} \pi q$$

Out[71]=

$$-\frac{\pi \text{rh}\theta^4}{16} +$$

$$\left( \pi \in (-297 c_1 q^4 - 648 c_2 q^4 - 1296 c_3 q^4 - 648 c_4 q^4 - 108 c_1 q^2 \text{rh}\theta^4 + 864 c_2 q^2 \text{rh}\theta^4 + 720 c_1 \text{rh}\theta^8 + 33 c_1 q^2 \text{rh}\theta^6 \Lambda e - 324 c_1 \text{rh}\theta^{10} \Lambda e + 28 c_1 \text{rh}\theta^{12} \Lambda e^2) \right) /$$

$$(72 \text{rh}\theta^2 (-15 q^2 + 12 \text{rh}\theta^4 + 4 \text{rh}\theta^6 \Lambda e))$$

Out[72]=

$$-\frac{1}{2304 \text{rh}\theta^8} \pi (216 (3 (2 c_3 + c_4) q^4 + c_2 (3 q^4 - 8 q^2 \text{rh}\theta^4)) + c_1 (387 q^4 + 192 q^2 \text{rh}\theta^4 (-9 + \text{rh}\theta^2 \Lambda e) + 16 \text{rh}\theta^8 (324 - 120 \text{rh}\theta^2 \Lambda e + 7 \text{rh}\theta^4 \Lambda e^2)))$$

Note that the above thermodynamic quantities can be expressed using any of the sets of variables : {rh, q,  $\Lambda e$ ,  $\epsilon$ }, {rh, q,  $\Lambda$ ,  $\epsilon$ }, {rh0, q,  $\Lambda e$ ,  $\epsilon$ }, or {rh0, q,  $\Lambda$ ,  $\epsilon$ }, by simply using the following substitutions : rh -> rhf, rh0 -> rh0f,  $\Lambda e$  ->  $\Lambda e f$ , and  $\Lambda$  ->  $\Lambda f$ .

Besides, for extremal BH with  $T=0$ , the conjugate quantity associated to  $\epsilon$  can be obtained as follows:

In[74]=

```
tem == 0;
Solve[%, q]
```

Out[75]=

$$\left\{ \left\{ q \rightarrow -\frac{2 \sqrt{3 \text{rh}\theta^4 - \text{rh}\theta^6 \Lambda e}}{\sqrt{3}} \right\}, \left\{ q \rightarrow \frac{2 \sqrt{3 \text{rh}\theta^4 - \text{rh}\theta^6 \Lambda e}}{\sqrt{3}} \right\} \right\}$$

In[76]=

$$\text{vthEp} /. q \rightarrow \frac{2 \sqrt{3 \text{rh}\theta^4 - \text{rh}\theta^6 \Lambda e}}{\sqrt{3}} /. \Lambda e \rightarrow -6 / \text{le}^2 // \text{Simplify} // \text{sr}$$

Out[76]=

$$-\frac{1}{16 \text{le}^4} \pi (c_1 (31 \text{le}^4 + 124 \text{le}^2 \text{rh}\theta^2 + 136 \text{rh}\theta^4) + 24 (\text{le}^2 + 2 \text{rh}\theta^2) (3 (2 c_3 + c_4) (\text{le}^2 + 2 \text{rh}\theta^2) + c_2 (\text{le}^2 + 6 \text{rh}\theta^2)))$$

## 6.The red-shifted free energy and the weak gravity conjecture.

The redshift factor is:

In[78]:=  $\lambda f = \sqrt{\Lambda e f / \Lambda} // \text{sr}$

Out[78]=  $1 - \frac{c1 \epsilon \Lambda}{18}$

For the redshifted BH, the conjugate quantity  $\tilde{\Theta}$  associated to  $\Lambda$  is given by

In[79]:= `tem /  $\lambda f$  /.  $\Lambda e \rightarrow \Lambda e f$  // sr;  
D[(% /.  $\text{rh}\theta \rightarrow \text{rh}\theta[\Lambda]$ ),  $\Lambda$ ] // sr;  
Solve[% == 0,  $\text{rh}\theta'[\Lambda]$ ] /.  $\text{rh}\theta[\Lambda] \rightarrow \text{rh}\theta$ ;  
jacL =  $\text{rh}\theta'[\Lambda]$  /. %[[1]] // sr;  
freeRed = freeqtPd /  $\lambda f$  /.  $\Lambda e \rightarrow \Lambda e f$  // sr;  
D[freeRed,  $\Lambda$ ] + D[freeRed,  $\text{rh}\theta$ ] * jacL;  
vth $\Delta$ Red = % /.  $k1 \rightarrow 1$  // sr`

Out[85]= 
$$-\frac{\pi \text{rh}\theta^4}{16} + \frac{(\epsilon (-807 c1 \pi q^4 - 1728 c2 \pi q^4 - 3456 c3 \pi q^4 - 1728 c4 \pi q^4 - 336 c1 \pi q^2 \text{rh}\theta^4 + 2304 c2 \pi q^2 \text{rh}\theta^4 + 1968 c1 \pi \text{rh}\theta^8 + 72 c1 \pi q^2 \text{rh}\theta^6 \Lambda - 832 c1 \pi \text{rh}\theta^{10} \Lambda + 80 c1 \pi \text{rh}\theta^{12} \Lambda^2))}{(192 \text{rh}\theta^2 (-15 q^2 + 12 \text{rh}\theta^4 + 4 \text{rh}\theta^6 \Lambda))}$$

For the redshifted BH, the conjugate quantity  $\tilde{U}_\epsilon$  associated to  $\epsilon$  is given by

In[87]:= `tem /  $\lambda f$  /.  $\Lambda e \rightarrow \Lambda e f$  // sr;  
Coefficient[D[(% /.  $\text{rh}\theta \rightarrow \text{rh}\theta[\epsilon]$ ),  $\epsilon$ ],  $\epsilon$ , 0];  
Solve[% == 0,  $\text{rh}\theta'[\epsilon]$ ] /.  $\text{rh}\theta[\epsilon] \rightarrow \text{rh}\theta$ ;  
jacL =  $\text{rh}\theta'[\epsilon]$  /. %[[1]];  
freeRed = freeqtPd /  $\lambda f$  /.  $\Lambda e \rightarrow \Lambda e f$  // sr;  
D[freeRed,  $\epsilon$ ] + D[freeRed,  $\text{rh}\theta$ ] * jacL;  
vthGaRed = % /.  $k1 \rightarrow 1$  // sr`

Out[93]= 
$$\frac{1}{2304 \text{rh}\theta^8} (-387 c1 \pi q^4 - 648 c2 \pi q^4 - 1296 c3 \pi q^4 - 648 c4 \pi q^4 + 1728 c1 \pi q^2 \text{rh}\theta^4 + 1728 c2 \pi q^2 \text{rh}\theta^4 - 5184 c1 \pi \text{rh}\theta^8 - 180 c1 \pi q^2 \text{rh}\theta^6 \Lambda + 1968 c1 \pi \text{rh}\theta^{10} \Lambda - 104 c1 \pi \text{rh}\theta^{12} \Lambda^2)$$

The verification of the first law for the redshifted BH:

```
In[94]:= diff[tquant_] := Outer[D, {tquant}, {rh0, q, Δ, ε}];
diff[sr[massPd / λf /. Δe → Δef]] -
  sr[(tem / λf /. Δe → Δef)] * diff[sr[entrPd /. Δe → Δef]] -
  sr[(phiPd / λf /. Δe → Δef)] diff[Q0] - vthΔRed * diff[Δ] -
  vthGaRed * diff[ε] // sr;
Table[%[[1]][[i]] == 0, {i, 1, 3}]
Series[%[[1]][[4]], {ε, 0, 0}] == 0 // Simplify
```

```
Out[96]:= {True, True, True}
```

```
Out[97]:= True
```

( $\tilde{U}_\epsilon d\epsilon$  is at first order in  $\epsilon$ , so  $\tilde{U}_\epsilon$  should be understood at zero order in  $\epsilon$ .)

The weak gravity conjecture concerns about  $d\tilde{M}/d\epsilon$  at the extremal temperature  $T=0$ . According to our analysis in the paper, it is given by  $\lim_{T \rightarrow 0} \tilde{U}_\epsilon$ .

```
In[98]:= tem == 0;
Solve[%, q]
```

```
Out[99]:= {{q -> -\frac{2 \sqrt{3 rh0^4 - rh0^6 Δe}}{\sqrt{3}}}, {q -> \frac{2 \sqrt{3 rh0^4 - rh0^6 Δe}}{\sqrt{3}}}}
```

```
In[102]:= vthGaRed /. q -> \frac{2 \sqrt{3 rh0^4 - rh0^6 Δe}}{\sqrt{3}} /. Δe -> Δef /. Δ -> -6 / l^2 // sr0
Coefficient[%, c1] * c1 // Simplify
```

```
Out[102]:= \frac{1}{16 l^4} (-31 c1 l^4 \pi - 24 c2 l^4 \pi - 144 c3 l^4 \pi - 72 c4 l^4 \pi -
128 c1 l^2 \pi rh0^2 - 192 c2 l^2 \pi rh0^2 - 576 c3 l^2 \pi rh0^2 - 288 c4 l^2 \pi rh0^2 -
138 c1 \pi rh0^4 - 288 c2 \pi rh0^4 - 576 c3 \pi rh0^4 - 288 c4 \pi rh0^4)
```

```
Out[103]:= -\frac{c1 \pi (31 l^4 + 128 l^2 rh0^2 + 138 rh0^4)}{16 l^4}
```

\* More on Example II: The calculation of the thermodynamic quantities from the traditional approach. The results verify those obtained from the simple approach.



By traditional approach, we mean to start from the perturbed BH solution due to the higher derivative terms, and to use the standard techniques based on the metric to calculate the thermodynamic quantities.

In[106]:= **Quit[]**

## 0. The perturbed BH solution.

The perturbed BH solution in D=5 dimensions can be found in arXiv:1912.11161, which is

In[1]:= **metric = DiagonalMatrix[**  

$$\{- (f[r]), 1 / (h[r]), r^2, r^2 * (\text{Sin}[\psi])^2, r^2 * (\text{Sin}[\psi] * \text{Sin}[\theta])^2\}];$$

In[2]:= **coord = {t, r,  $\psi$ ,  $\theta$ ,  $\phi$ };**  
**\$Assumptions = And[t  $\in$  Reals, M  $\in$  Reals,**  

$$r \in \text{Reals}, r > 0, 0 < \phi < 2\pi, 0 < \psi < \pi, 0 < \theta < \pi, M > 0, \Lambda < 0];$$
  
**metricsign = -1;**  
**<< "D:\\diffgeoM.wl"**  
**rie0 = lower[Riemann, {4}];**

In[7]:= **g1[r\_] =**  

$$1 + \frac{q^2}{4 r^4} - \frac{\mu}{r^2} + \frac{r^2}{l^2} + \frac{1}{96 l^2 r^{10}} \left( -191 c1 l^4 q^4 - 216 c2 l^4 q^4 - 144 c3 l^4 q^4 - 72 c4 l^4 q^4 + \right.$$

$$992 c1 l^4 \mu q^2 r^2 + 960 c2 l^4 \mu q^2 r^2 + 192 c1 l^4 \mu^2 r^4 - 1536 c1 l^4 q^2 r^4 -$$

$$1152 c2 l^4 q^2 r^4 - 2080 c1 l^2 q^2 r^6 - 1728 c2 l^2 q^2 r^6 + 64 c1 r^{12} \left. \right) \epsilon;$$

$$f1[r_] = 1 + \frac{q^2}{4 r^4} - \frac{\mu}{r^2} + \frac{r^2}{l^2} + \frac{1}{96 l^2 r^{10}} \left( 17 c1 l^4 q^4 - 24 c2 l^4 q^4 - 144 c3 l^4 q^4 - \right.$$

$$72 c4 l^4 q^4 + 160 c1 l^4 \mu q^2 r^2 + 192 c2 l^4 \mu q^2 r^2 + 192 c1 l^4 \mu^2 r^4 -$$

$$704 c1 l^4 q^2 r^4 - 384 c2 l^4 q^2 r^4 - 1248 c1 l^2 q^2 r^6 - 960 c2 l^2 q^2 r^6 + 64 c1 r^{12} \left. \right) \epsilon;$$
**sr[var\_] := Normal[Series[var, { $\epsilon$ , 0, 1}]];**

The perturbed solution for the electromagnetic sector is given by

In[10]:= **au =**  

$$\left\{ -\frac{\sqrt{3} q}{2 r^2} + \frac{1}{24 r^8} \left( -13 \sqrt{3} c1 l^2 q^3 + 48 \sqrt{3} c2 l^2 q^3 + 144 \sqrt{3} c3 l^2 q^3 + 72 \sqrt{3} c4 l^2 q^3 - \right. \right.$$

$$96 \sqrt{3} c2 l^2 \mu q r^2 + 96 \sqrt{3} c2 q r^6 \left. \right) \epsilon, 0, 0, 0, 0 \};$$

In[11]:=

fuv =

$$\left\{ \left\{ 0, -\frac{\sqrt{3} q}{r^3} + \frac{1}{3 r^9} \left( -13 \sqrt{3} c_1 l^2 q^3 + 48 \sqrt{3} c_2 l^2 q^3 + 144 \sqrt{3} c_3 l^2 q^3 + 72 \sqrt{3} c_4 l^2 q^3 - 72 \sqrt{3} c_2 l^2 \mu q r^2 + 24 \sqrt{3} c_2 q r^6 \right) \epsilon, 0, 0, 0 \right\}, \right. \\ \left. \left\{ \frac{\sqrt{3} q}{r^3} + \frac{1}{3 r^9} \left( 13 \sqrt{3} c_1 l^2 q^3 - 48 \sqrt{3} c_2 l^2 q^3 - 144 \sqrt{3} c_3 l^2 q^3 - 72 \sqrt{3} c_4 l^2 q^3 + 72 \sqrt{3} c_2 l^2 \mu q r^2 - 24 \sqrt{3} c_2 q r^6 \right) \epsilon, \right. \right. \\ \left. \left. 0, 0, 0, 0 \right\}, \{0, 0, 0, 0, 0\}, \{0, 0, 0, 0, 0\}, \{0, 0, 0, 0, 0\} \right\};$$

1. The calculations for the temperature, electromagnetic potential and electric charge. All of them are expressed as the functions of the horizon radius  $rh$  and the electric charge  $q$ .

First calculate the mass parameter  $\mu$  in the metric and its expression  $\mu_h$ . Note that  $\mu$  is not the thermodynamic energy of the BH, but simply a parameter related to the energy.

In[12]:=

$$\text{f1}[rh] /. \mu \rightarrow \frac{q^2}{4 rh^2} + rh^2 + \frac{rh^4}{l^2} + \epsilon b1 // \text{sr};$$

$$\text{Solve}[\% == 0, b1];$$

$$\mu_h = \frac{q^2}{4 rh^2} + rh^2 + \frac{rh^4}{l^2} + \epsilon b1 /. \%[[1]]$$

Out[14]=

$$\frac{q^2}{4 rh^2} + rh^2 + \frac{rh^4}{l^2} + \frac{1}{96 l^2 rh^8} \\ \left( 69 c_1 l^4 q^4 + 24 c_2 l^4 q^4 - 144 c_3 l^4 q^4 - 72 c_4 l^4 q^4 - 448 c_1 l^4 q^2 rh^4 - 192 c_2 l^4 q^2 rh^4 - \right. \\ \left. 992 c_1 l^2 q^2 rh^6 - 768 c_2 l^2 q^2 rh^6 + 192 c_1 l^4 rh^8 + 384 c_1 l^2 rh^{10} + 256 c_1 rh^{12} \right) \epsilon$$

The expression of the temperature (denoted as  $tem$ ):

In[15]:=

```
1 / (4 Pi) Sqrt[D[f[r], r] * D[h[r], r]] /. {f -> f1, h -> g1} // sr;
% /. r -> rh /. mu -> muh // Simplify // sr;

tem = % /. Sqrt[(-1^2 q^2 + 4 l^2 rh^4 + 8 rh^6)^2 / 1^4] -> (-1^2 q^2 + 4 l^2 rh^4 + 8 rh^6) / 1^2 // Simplify // sr
```

Out[17]:=

$$-\frac{q^2}{8\pi rh^5} + \frac{1}{2\pi rh} + \frac{rh}{l^2\pi} + \frac{1}{48l^2\pi rh^{11}} \\ (-27c_1l^4q^4 + 12c_2l^4q^4 + 144c_3l^4q^4 + 72c_4l^4q^4 + 80c_1l^4q^2rh^4 - 48c_2l^4q^2rh^4 - \\ 64c_1l^2q^2rh^6 - 96c_2l^2q^2rh^6 - 96c_1l^4rh^8 - 192c_1l^2rh^{10} - 64c_1rh^{12}) \in$$

The expression for the electrostatic potential (denoted as [phih](#)):

In[18]:=

```
phih = -au[[1]] /. r -> rh // sr;
phih = % /. mu -> muh // sr
```

Out[19]:=

$$\frac{\sqrt{3}q}{2rh^2} + \frac{1}{24rh^8} \\ (13\sqrt{3}c_1l^2q^3 - 24\sqrt{3}c_2l^2q^3 - 144\sqrt{3}c_3l^2q^3 - 72\sqrt{3}c_4l^2q^3 + 96\sqrt{3}c_2l^2qrh^4) \in$$

The expression of the electric charge (denoted as [qh](#)):

In[20]:=

```
ff2 = contract[fuv ** fuv, {1, 3}, {2, 4}] // sr;
ff3 = Transpose[contract[fuv ** fuv ** fuv, {2, 3}, {4, 5}], {1, 2}] // sr;
fuvHighC =
  e l^2 (-4 c2 contract[rie0 ** fuv, {3, 5}, {4, 6}] - 8 c3 fuv ff2 - 8 c4 ff3) /.
  {f -> f1, h -> g1} // sr;
fuvF1 = fuv + fuvHighC // sr;
```

In[24]:=

```
fuvF1[[2, 1]] * Sqrt[f1[r] / g1[r]] * 2 Pi^2 r^3 // sr;
qh = Limit[%, (16 Pi), r -> Infinity]
```

Out[25]:=

$$\frac{1}{8} \sqrt{3} \pi q$$

## 2. The expression of BH energy and entropy from the Euclidean action

In the traditional approach, the Euclidean action is calculated from the perturbed solution.

(1) The part  $\int R + \frac{12}{l^2} - \frac{1}{4} F^2$  of the Euclidean action.

In[26]:=

```
( (RicciScalar + 12 / l^2) * Sqrt[f1[r] / g1[r]] /. {f -> f1, h -> g1} ) * 2 Pi^2 r^3 // sr;
intR[r_] = (Integrate[%, r]) // sr;
- contract[1 / 4 fuv ** fuv, {1, 3}, {2, 4}] * 2 Pi^2 r^3 * Sqrt[f[r] / h[r]] /.
{f -> f1, h -> g1} // Simplify // sr;
intEm[r_] = Integrate[%, r] // Simplify // sr;
int[r_] = intR[r] + intEm[r];
int[rt] - int[rh] // Simplify // sr;
rInt = % /. {f -> f1, h -> g1} // Simplify // sr
```

Out[31]=

$$\frac{\pi^2 \left( -l^2 q^2 rh^2 + l^2 q^2 rt^2 + 4 rh^6 rt^2 - 4 rh^2 rt^6 \right)}{l^2 rh^2 rt^2} + \frac{1}{48 rh^8 rt^8}$$

$$\pi^2 \left( -864 c1 l^2 \mu q^2 rh^8 rt^2 - 1728 c2 l^2 \mu q^2 rh^8 rt^2 + 384 c1 l^2 q^2 rh^8 rt^4 + \right.$$

$$1152 c2 l^2 q^2 rh^8 rt^4 + 2080 c1 q^2 rh^8 rt^6 + 3264 c2 q^2 rh^8 rt^6 + 864 c1 l^2 \mu q^2 rh^2 rt^8 +$$

$$1728 c2 l^2 \mu q^2 rh^2 rt^8 - 384 c1 l^2 q^2 rh^4 rt^8 - 1152 c2 l^2 q^2 rh^4 rt^8 - 2080 c1 q^2 rh^6 rt^8 -$$

$$3264 c2 q^2 rh^6 rt^8 + 3 (57 c1 + 200 c2 + 240 c3 + 120 c4) l^2 q^4 (rh^8 - rt^8) + \frac{1}{l^2}$$

$$\left. 64 (9 c1 l^4 \mu^2 rh^8 rt^4 - 9 c1 l^4 \mu^2 rh^4 rt^8 + 5 c1 rh^{12} rt^8 - 5 c1 rh^8 rt^{12}) \right) \in$$

Compute the factor  $\sqrt{g_{tt}(\text{BH})/g_{tt}(\text{AdS})}$  (denoted as [m12b](#) below) needed in the background subtraction, which is a technique to regularize the divergences.

In[32]:=

```
f1[r] / (f1[r] /. {mu -> 0, q -> 0});
Sqrt[%] /. r -> 1 / ep;
Series[%, {ep, 0, 6}] // Normal;
m12b = % /. ep -> 1 / rt // sr
```

Out[35]=

$$\frac{4 l^4 \mu + l^2 q^2 - 4 l^2 \mu rt^2 + 8 rt^6}{8 rt^6} + \frac{(-8 c1 l^4 \mu - 79 c1 l^2 q^2 - 60 c2 l^2 q^2 + 4 c1 l^2 \mu rt^2)}{12 rt^6} \in$$

The regularized result of  $\int R + \frac{12}{l^2} - \frac{1}{4} F^2$  :

```
In[36]:= rInt - m12b (int[rt] /. {mu -> 0, q -> 0}) // Simplify;
1 / (16 Pi) Limit[%, rt -> Infinity] // Expand;
lnzLowC = beta % /. mu -> muh // sr
```

Out[38]=

$$\frac{\pi q^2 \beta}{32 rh^2} - \frac{1}{8} \pi rh^2 \beta + \frac{\pi rh^4 \beta}{8 l^2} + \frac{1}{192 l^2 rh^8} \left( -15 c1 l^4 \pi q^4 \beta - 48 c2 l^4 \pi q^4 \beta - 144 c3 l^4 \pi q^4 \beta - 72 c4 l^4 \pi q^4 \beta + 160 c1 l^4 \pi q^2 rh^4 \beta + 192 c2 l^4 \pi q^2 rh^4 \beta - 134 c1 l^2 \pi q^2 rh^6 \beta - 192 c2 l^2 \pi q^2 rh^6 \beta - 192 c1 l^4 \pi rh^8 \beta - 408 c1 l^2 \pi rh^{10} \beta - 152 c1 \pi rh^{12} \beta \right) \in$$

## (2) The higher curvature part of the Euclidean action:

```
In[39]:= contract[rie0**rie0, {3, 5}, {4, 6}];
rHc1 = contract[%, {1, 3}, {2, 4}] /. {f -> f1, h -> g1} // sr;
rie0**fuv**fuv;
rHc2 = contract[%, {1, 5}, {2, 6}, {3, 7}, {4, 8}] /. {f -> f1, h -> g1} // sr;
fuv**fuv;
contract[%, {1, 3}, {2, 4}] /. {f -> f1, h -> g1};
rHc3 = %^2 // sr;
fuvup = raise[fuv, {1, 2}] // sr;
((fuv.fuvup).fuv).fuvup;
rHc4 = tr[%, {1, 2}] /. {f -> f1, h -> g1} // sr;
e1^2 (c1 rHc1 + c2 rHc2 + c3 rHc3 + c4 rHc4) // Simplify;
ind = % // sr // Simplify;
(ind) * 2 Pi^2 r^3 * Sqrt[f1[r] / g1[r]] /. {f -> f1, h -> g1} // sr;
int[r_] = Integrate[%, r] // sr;
int[rt] - int[rh] // Simplify;
rInt = % // Simplify // sr
```

Out[54]=

$$-\frac{1}{16 l^2 rh^8 rt^8} \pi^2 \left( 72 (2 c3 + c4) l^4 q^4 (rh^8 - rt^8) - 24 c2 l^2 q^2 (-8 rh^8 rt^6 + 8 rh^6 rt^8 + l^2 (8 mu rh^2 rt^2 (rh^6 - rt^6) - 5 q^2 (rh^8 - rt^8))) + c1 (32 l^2 q^2 rh^6 rt^6 (rh^2 - rt^2) + 320 rh^8 rt^8 (rh^4 - rt^4) + l^4 (576 mu^2 rh^4 rt^4 (rh^4 - rt^4) - 480 mu q^2 rh^2 rt^2 (rh^6 - rt^6) + 127 q^4 (rh^8 - rt^8))) \right) \in$$

```
In[55]:= rInt - m12b (int[rt] /. {mu -> 0, q -> 0}) // Simplify // sr;
Limit[%, rt -> Infinity] // Expand;
lnzHighC = 1 / (16 Pi) * beta % // sr
```

```
Out[57]=
```

$$\frac{1}{256 l^2 r h^8} \left( 127 c_1 l^4 \pi q^4 \beta + 120 c_2 l^4 \pi q^4 \beta + 144 c_3 l^4 \pi q^4 \beta + 72 c_4 l^4 \pi q^4 \beta - 480 c_1 l^4 \mu \pi q^2 r h^2 \beta - 192 c_2 l^4 \mu \pi q^2 r h^2 \beta + 576 c_1 l^4 \mu^2 \pi r h^4 \beta + 32 c_1 l^2 \pi q^2 r h^6 \beta + 192 c_2 l^2 \pi q^2 r h^6 \beta + 160 c_1 l^2 \mu \pi r h^8 \beta - 320 c_1 \pi r h^{12} \beta \right) \in$$

(3) The total free energy, and other thermodynamic quantities followed from it.

```
In[58]:= free = - (lnzLowC + lnzHighC) / beta /. mu -> muh // sr
```

```
Out[58]=
```

$$-\frac{\pi q^2}{32 r h^2} + \frac{\pi r h^2}{8} - \frac{\pi r h^4}{8 l^2} + \frac{1}{768 l^2 r h^8} \left( -69 c_1 l^4 \pi q^4 - 24 c_2 l^4 \pi q^4 + 144 c_3 l^4 \pi q^4 + 72 c_4 l^4 \pi q^4 - 64 c_1 l^4 \pi q^2 r h^4 - 192 c_2 l^4 \pi q^2 r h^4 + 896 c_1 l^2 \pi q^2 r h^6 + 768 c_2 l^2 \pi q^2 r h^6 - 960 c_1 l^4 \pi r h^8 - 2304 c_1 l^2 \pi r h^{10} - 640 c_1 \pi r h^{12} \right) \in$$

This free energy is that of an ensemble depending on  $T$  and  $\phi$ . We can turn to another kind of free energy depending on  $T$  and  $q$ , through a Legendre Transformation.

```
In[60]:= freeqt = free + qh * phih /. mu -> muh // sr
```

```
Out[60]=
```

$$\frac{5 \pi q^2}{32 r h^2} + \frac{\pi r h^2}{8} - \frac{\pi r h^4}{8 l^2} + \frac{1}{768 l^2 r h^8} \left( 87 c_1 l^4 \pi q^4 - 312 c_2 l^4 \pi q^4 - 1584 c_3 l^4 \pi q^4 - 792 c_4 l^4 \pi q^4 - 64 c_1 l^4 \pi q^2 r h^4 + 960 c_2 l^4 \pi q^2 r h^4 + 896 c_1 l^2 \pi q^2 r h^6 + 768 c_2 l^2 \pi q^2 r h^6 - 960 c_1 l^4 \pi r h^8 - 2304 c_1 l^2 \pi r h^{10} - 640 c_1 \pi r h^{12} \right) \in$$

Calculate the entropy from the formula  $S = dF / dT$ :

```
In[61]:= entr = -D[freeqt, rh] / D[tem, rh] // sr
```

```
Out[61]=
```

$$\frac{\pi^2 r h^3}{2} - \frac{\pi^2 (7 c_1 l^2 q^2 + 6 c_2 l^2 q^2 - 12 c_1 l^2 r h^4 - 8 c_1 r h^6)}{2 r h^3} \in$$

For cross-checking, we can also calculate the entropy from the Wald entropy, which is a method independent of the Euclidean method.

In[62]:=

```
entrWd = 2 Pi^2 rh^3 / 4
  ( 1 - ε * l^2 ( 4 c1 rie0[[1, 2, 1, 2]] + 2 c2 fuv[[1, 2]] fuv[[1, 2]] ) ) /.
  {f -> f1, h -> g1} /. r -> rh // sr
entr == entrWd /. mu -> muh //
sr
```

Out[62]=

$$\frac{\pi^2 rh^3}{2} + \frac{(-5 c1 l^2 \pi^2 q^2 - 3 c2 l^2 \pi^2 q^2 + 6 c1 l^2 \mu \pi^2 rh^2 - 2 c1 \pi^2 rh^6) \epsilon}{rh^3}$$

Out[63]=

True

The energy of the BH is calculated from the formula  $M=F+TS$ :

In[64]:=

```
massh = freeqt + tem * entr // sr
```

Out[64]=

$$\frac{3 \pi q^2}{32 rh^2} + \frac{3 \pi rh^2}{8} + \frac{3 \pi rh^4}{8 l^2} + \frac{1}{256 l^2 rh^8} \\ (69 c1 l^4 \pi q^4 + 24 c2 l^4 \pi q^4 - 144 c3 l^4 \pi q^4 - 72 c4 l^4 \pi q^4 - 448 c1 l^4 \pi q^2 rh^4 - \\ 192 c2 l^4 \pi q^2 rh^4 - 896 c1 l^2 \pi q^2 rh^6 - 768 c2 l^2 \pi q^2 rh^6 + \\ 192 c1 l^4 \pi rh^8 + 768 c1 l^2 \pi rh^{10} + 640 c1 \pi rh^{12}) \epsilon$$

The relation between  $M$  and the mass parameter  $\mu$  in the metric.

In[65]:=

```

$$\frac{3 \pi}{8} (1 + \epsilon b2) \mu h - massh // sr;$$

Solve[% == 0, b2];
massMu = 
$$\frac{3 \pi}{8} (1 + \epsilon b2) \mu /. \%[[1]]$$

```

Out[67]=

$$\frac{3}{8} \mu \pi (1 + 4 c1 \epsilon)$$

### 3. The comparison of the results from the traditional approach to those from the simple approach.

Before doing comparison, we should make the substitution  $\epsilon \rightarrow \epsilon l^2$  in the results of the simple approach (the factor is merely caused by the difference in convention).

Notice that the relation between the AdS radius  $l$  and effective AdS radius  $le$  is given by

```
In[68]:= f1[r] /. {q -> 0, mu -> 0};
1 +  $\frac{r^2}{l^2} + \frac{2 c1 r^2 \epsilon}{3 l^2} == 1 + \frac{r^2}{le^2} /. le \rightarrow (1 + \epsilon b2) l // sr;$ 
Solve[%, b2];
lef = (1 +  $\epsilon b2$ ) l /. %[[1]]
lf = (1 -  $\epsilon b2$ ) le /. %%[[1]]
```

```
Out[71]= l  $\left(1 - \frac{c1 \epsilon}{3}\right)$ 
```

```
Out[72]= le  $\left(1 + \frac{c1 \epsilon}{3}\right)$ 
```

(Thus we can change the variable from  $le$  to  $l$ , or from  $l$  to  $le$ , by using the substitution  $le \rightarrow lef$  or  $l \rightarrow lf$ .)

The relation between  $rh$  and  $rh0$  ( $\bar{rh}$  in the paper) is given below:

```
In[73]:= temLe = tem /. l -> lf // sr;
temLe -  $\left(-\frac{q^2}{8 \pi rh0^5} + \frac{1}{2 \pi rh0} + \frac{rh0}{le^2 \pi}\right) /. rh \rightarrow rh0 + \epsilon b1 // sr;$ 
Solve[% == 0, b1];
rhf = rh0 +  $\epsilon b1$  /. %[[1]]
```

```
Out[76]= rh0 +  $\left(\left(27 c1 le^4 q^4 - 12 c2 le^4 q^4 - 144 c3 le^4 q^4 - 72 c4 le^4 q^4 - 80 c1 le^4 q^2 rh0^4 + 48 c2 le^4 q^2 rh0^4 + 64 c1 le^2 q^2 rh0^6 + 96 c2 le^2 q^2 rh0^6 + 96 c1 le^4 rh0^8 + 192 c1 le^2 rh0^{10} + 96 c1 rh0^{12}\right) \epsilon\right) / \left(6 rh0^5 \left(5 le^2 q^2 - 4 le^2 rh0^4 + 8 rh0^6\right)\right)$ 
```

Using the substitution  $rh \rightarrow rhf$  and  $l \rightarrow lf$ , we can re-express the free energy, mass, entropy and electrostatic potential using the variables  $rh0$  and  $le$ .

Indeed, these results coincides with those obtained from the simple approach.

For example, we can compare  $entr$  (derived from the traditional approach) and  $entrPd$  (derived from the simple approach) :



In[77]:=

```
entr /. {l → lf, rh → rhf} // sr;
entrPd =

$$\frac{\pi^2 \text{rh}\theta^3}{2} + \left( \pi^2 \epsilon \left( 387 c_1 q^4 + 648 c_2 q^4 + 1296 c_3 q^4 + 648 c_4 q^4 - 864 c_1 q^2 \text{rh}\theta^4 - 864 c_2 q^2 \text{rh}\theta^4 + 48 c_1 q^2 \text{rh}\theta^6 \Lambda e + 480 c_1 \text{rh}\theta^{10} \Lambda e - 56 c_1 \text{rh}\theta^{12} \Lambda e^2 \right) \right) /$$


$$\left( -180 q^2 \text{rh}\theta^3 + 48 \text{rh}\theta^7 (3 + \text{rh}\theta^2 \Lambda e) \right) /. \epsilon \rightarrow 1 e^2 \epsilon /. \Lambda e \rightarrow -6 / 1 e^2 // sr;$$

% ==
%% //
Simplify
```

Out[79]=

True

And compare [phi<sub>h</sub>](#) (derived from the traditional approach) and [phi<sub>Pd</sub>](#) (derived from the simple approach) :

In[80]:=

```
phih /. {l → lf, rh → rhf} // sr;
phiPd =

$$\frac{\sqrt{3} q}{2 \text{rh}\theta^2} + \left( \epsilon \left( 129 c_1 q^5 + 216 c_2 q^5 + 432 c_3 q^5 + 216 c_4 q^5 - 804 c_1 q^3 \text{rh}\theta^4 - 1152 c_2 q^3 \text{rh}\theta^4 - 1728 c_3 q^3 \text{rh}\theta^4 - 864 c_4 q^3 \text{rh}\theta^4 + 1152 c_1 q \text{rh}\theta^8 + 1152 c_2 q \text{rh}\theta^8 - 76 c_1 q^3 \text{rh}\theta^6 \Lambda e - 288 c_2 q^3 \text{rh}\theta^6 \Lambda e - 576 c_3 q^3 \text{rh}\theta^6 \Lambda e - 288 c_4 q^3 \text{rh}\theta^6 \Lambda e - 384 c_1 q \text{rh}\theta^{10} \Lambda e + 384 c_2 q \text{rh}\theta^{10} \Lambda e + 32 c_1 q \text{rh}\theta^{12} \Lambda e^2 \right) \right) /$$


$$\left( 8 \sqrt{3} \text{rh}\theta^8 (-15 q^2 + 12 \text{rh}\theta^4 + 4 \text{rh}\theta^6 \Lambda e) \right) /. \epsilon \rightarrow 1 e^2 \epsilon /. \Lambda e \rightarrow -6 / 1 e^2 // sr;$$

% == %% // FullSimplify
```

Out[82]=

True

We also examined all the thermodynamic quantities including the conjugate quantities associated with [α](#) and [Λ](#). All the results have been nicely verified.
